# Supplementary material for: Crossmodal Attentive Skill Learner
Source: arXiv:1711.10314 source file (2018-05-22)
Supplement: Supplementary file 1 [file supplemental.tex]

\onecolumn
\pagebreak

\begin{center}
	\textbf{\large Supplemental Material}
\end{center}
